# Supplementary material for: GFM4MPM: Towards Geospatial Foundation Models for Mineral Prospectivity Mapping
Source: arXiv:2406.12756 source file (2024-06-18)
Supplement: Supplementary file 1 [file additional_text.tex]

Evaluating the performance of a classification model is crucial for understanding its effectiveness, robustness, and generality. However, various metrics can provide different perspectives on how well the model performs. We evaluate our models on several widely used metrics including 
\textbf{F1-score}, 
\textbf{A}rea \textbf{U}nder the \textbf{R}eceiver \textbf{O}perating \textbf{C}haracteristic Curve (\textbf{AUROC}), 
\textbf{A}rea \textbf{U}nder the \textbf{P}recision-\textbf{R}ecall \textbf{C}urve (\textbf{AUPRC}), \textbf{Acc}uracy (\textbf{ACC}),
\textbf{B}alanced \textbf{Acc}uracy (\textbf{B.ACC}), and 
\textbf{M}atthews \textbf{C}orrelation \textbf{C}oefficient (\textbf{MCC}).

\textbf{Notation:} Below, we are going to rely on the following abbreviations: \textbf{TP} - True Positives, \textbf{TN} - True Negatives, \textbf{FP} - False Positives, and \textbf{FN} - False Negatives, referring to the number of instances where the model correctly/incorrectly predicted the positive/negative classes.

\begin{enumerate}
    \item The \textbf{F1-score} is defined as the harmonic mean of \textit{Precision} and \textit{Recall}:
    \begin{equation}\label{eq:f1}
        \bm{F1}=\frac{2\cdot \bm{TP}}{2\cdot \bm{TP}+\bm{FP}+\bm{FN}}.
    \end{equation}
    It provides a balanced measure of a model's \textit{Precision} and \textit{Recall}, making it particularly useful for evaluating performance on imbalanced datasets where both \textbf{FP} and \textbf{FN} matter.
    
    \item The \textbf{AUROC} measures the ability of the model to distinguish between classes by plotting the \textbf{T}rue \textbf{P}ositive \textbf{R}ate (\textbf{TPR}) (also know as \textit{Sensitivity} or \textit{Recall}) against the \textbf{F}alse \textbf{P}ositive \textbf{R}ate (\textbf{FPR}) (i.e., \textit{1.0 - Specificity}):
    \begin{equation}\label{eq:auroc}
        \bm{AUROC}=\int_0^1 \bm{TPR}\left(\bm{FPR}^{-1}\left(x\right)\right) dx.
    \end{equation}
    The area under this curve indicates how well the model can distinguish between positive and negative classes.
    
    \item The \textbf{AUPRC} evaluates the trade-off between \textit{Precision} and \textit{Recall} for different thresholds:
    \begin{equation}\label{eq:auprc}
        \bm{AUPRC}=\int_0^1 Precision\left(Recall^{-1}\left(x\right)\right)dx.
    \end{equation}
    The area under the precision-recall curve reflects the model's performance across all recall levels, and can be particularly useful when working with imbalanced datasets.
    
    \item \textbf{ACC} measures the overall correctness of the model by calculating the proportion of true results (both \textbf{TP} and \textbf{TN}) among the total number of outcomes (i.e., \textbf{TP}, \textbf{TN}, \textbf{FP}, and \textbf{FN}):
    \begin{equation}\label{eq:acc}
        \bm{ACC}=\frac{\bm{TP}+\bm{TN}}{\bm{TP}+\bm{TN}+\bm{FP}+\bm{FN}}
    \end{equation}
    
    \item \textbf{B.ACC} is defined as an average of the \textbf{T}rue \textbf{P}ositive (\textbf{TPR}) and \textbf{T}rue \textbf{N}egative (\textbf{TNR}) rates:
    \begin{equation}\label{eq:b_acc}
        \bm{B.ACC}=\frac{1}{2}\left(\frac{\bm{TP}}{\bm{TP} + \bm{FN}} + \frac{\bm{TN}}{\bm{TN} + \bm{FP}} \right)
    \end{equation}
    Balanced Accuracy accounts for imbalanced class distributions and provides a more accurate measure of a model's performance across both classes. Alternatively, it can be interpreted as an average between the \textit{Recall} (or \textit{Sensitivity}) and \textit{Specificity}.
    
    \item The \textbf{MCC} is a comprehensive metric that considers all possible outcomes (i.e., \textbf{TP}, \textbf{TN}, \textbf{FP}, and \textbf{FN}) and provides a correlation coefficient between observed (i.e., ground truth) and predicted binary classifications:
    \begin{equation}\label{eq:mcc}
        \bm{MCC}=\frac{\bm{TP}\cdot \bm{TN}-\bm{FP}\cdot \bm{FN}}{\sqrt{(\bm{TP}+\bm{FP})(\bm{TP}+\bm{FN})(\bm{TN}+\bm{FP})(\bm{TN}+\bm{FN})}}.
    \end{equation}
\end{enumerate}

\subsection{Mineral Prospectivity Mapping}\label{ss:mpm}

\subsubsection{Mississippi Valley Type (MVT) Lead-Zinc deposits}\label{sss:mvt}

\begin{enumerate}
    \item Quantitative eval with ANOVA
    \item Qualitative plots of likelihood, uncertainty, feature attributions
\end{enumerate}

\subsubsection{Clastic-dominated (CD) Lead-Zinc deposits}\label{sss:cd}

\begin{enumerate}
    \item Quantitative eval with ANOVA
    \item Qualitative plots of likelihood, uncertainty, feature attributions
\end{enumerate}

\subsubsection{Mafic and Ultra-mafic Rock?}\label{sss:}

\begin{enumerate}
    \item Quantitative eval with ANOVA
    \item Qualitative plots of likelihood, uncertainty, feature attributions
\end{enumerate}

\subsection{Effect of SSL}\label{ss:effect_of_ssl}

\subsubsection{Computational Efficiency Analysis}\label{sss:computational_efficiency}

Quantitative table of FLOPS / size per model

\subsection{Effect of Likely Negative Sampling}\label{ss:effect_of_neg_sampling}

Metrics w/ vs w/out likely negative sampling at various ranges

ML for MPM remains a challenging problem as it requires the analysis of associations between large scale multi-modal geospatial data and few historical mineral commodity observations. The properties of geological mineralization have challenging implications for ML. First, mineralization is extremely rare, resulting in a highly imbalanced ML problem. Additionally, all remaining locations after excluding those with known presence of the exploration target are not necessarily absent at those locations (i.e., only positive labels are provided while negative labels are unknown). Second, domain knowledge of the geological mineralization processes continues to evolve as our understanding of geological processes improves. The set of geospatial explanatory features necessary to make accurate MPM predictions remains an active area of research. Third, explanatory features are multi-modal, spanning broad areas of geoscience (e.g., geology, geophysics, geochemistry). Therefore, validating individual ML MPM predictions can be challenging due to the multi-modal fusion and black-box nature of many ML systems. These aforementioned properties increase the uncertainties associated with ML MPM predictions.

We use the comprehensive set of explanatory feature layers compiled by~\cite{LAWLEY2022104635}. First, the set $m$ of explanatory feature layers should be selected. While selecting the explanatory feature layers most appropriate for a given mineral system and deposit type is fundamentally important for the success of MPM, we use the complete set of explanatory feature layers from~\cite{LAWLEY2022104635} shown in Table~\ref{} because selecting a sufficient, geologically relevant set is beyond the scope of this ML for MPM work \angel{remove and rephrase the previous sentence to make this text more assessment agnostic}.

Additionally, we confirmed whether differences observed mean prediction performances for each metric  were statistically significant using the Analysis of variance (ANOVA) test. When statistically significant differences were present, a post-hoc Tukey-HSD test was performed to identify which dependent variables differed (i.e. methods).
